# Supplementary material for: Physics-guided Learning-based Adaptive Control on the SE(3) Manifold
Source: arXiv:2201.04339 source file (2022-01-12)
Supplement: Supplementary file 1 [file Appendix.tex]

\section*{Appendix}
\label{sec:stability_proof}
In this section, we provide the stability analysis for our adaptive controller in Theorem \ref{thm:stability}.
\begin{theorem} \label{thm:stability}
	Consider the Hamiltonian dynamics in \eqref{eq:PH_dyn} with disturbance model in Sec. \ref{sec:problem_statement}. Suppose that the parameters $\bfg(\mathbf\frakq)$, $\bfM(\mathbf\frakq)$, $V(\mathbf\frakq)$, and $\bfW(\mathbf\frakq,\mathbf\frakp)$ are known but the distubance feature weights $\bfa^*$ are unknown. Let $\bfx^*(t)$, $t \geq t_0$ be a desired state trajectory with bounded angular velocity, $\|\bfomega^*(t)\| \leq \gamma$. Assume that the initial system state satisfies:
	\begin{equation}
	\begin{aligned}
	\tr(\bfI - \bfR^{*\top}(t_0)\bfR(t_0)) < \alpha < 2,\;
	\|\bfe_{\bfomega}(\bfx(t_0),\bfx^*(t_0))\| \leq \beta
	\end{aligned}
	\end{equation}
	for some constants $\alpha$, $\beta$. Consider the tracking controller in \eqref{eq:ES_DI_COMP_control} with adaptation law in \eqref{eq:geometric_adaptive_law}. Then, there exist positive constants $k_{\bfp}$, $k_{\bfR}$, $k_{\bfv}$, $k_{\bfomega}$, $c_{\bfp}$, $c_{\bfR}$, $c_{\bfv}$, $c_{\bfomega}$ such that the tracking errors $\bfe(\mathbf\frakq,\mathbf\frakq^*)$ and $\mathbf\frakp_e = \mathbf\frakp - \mathbf\frakp^*$ converge to zero. Also, the estimation error $\bfe_{\bfa} = \bfa - \bfa^*$ is stable in the sense of Lyapunov and uniformly bounded.
\end{theorem}

\begin{proof}
The stability analysis is developed in the domain $\calT = \crl{ \bfx \in TSE(3) \mid \tr(\bfI - \bfR^{*\top}\bfR) < \alpha < 2, \|\bfe_{\bfomega}(\bfx,\bfx^*)\| < \beta}$. Since $\tr(\bfI - \bfR^{*\top}\bfR) < \alpha < 2$, then $\|\bfe_{\bfR}\|_2^2 \leq \tr(\bfI - \bfR^{*\top}\bfR) \leq \frac{2}{2-\alpha} \|\bfe_{\bfR}\|_2^2$ by \cite[Prop.~1]{taeyoung2013robust}. We drop function parameters to simplify the notation. The derivative of the generalized coordinate error satisfies:
\begin{equation}
\begin{aligned} \label{eq:edot}
\dot{\bfe} &=  \begin{bmatrix}
  \dot{\bfe}_{\bfp} \\ \dot{\bfe}_{\bfR}
  \end{bmatrix} = \begin{bmatrix} -\hat{\bfomega} \bfe_{\bfp} + k_{\bfp}\bfe_{\bfv}\\
k_{\bfR}\bfE(\bfR,\bfR^*) \bfe_{\bfomega}
\end{bmatrix},\\
&= -\begin{bmatrix} \hat{\bfomega} & \mathbf{0}\\ \mathbf{0}& \mathbf{0} \end{bmatrix} \bfe + \begin{bmatrix} k_{\bfp} \bfI & \mathbf{0}\\\mathbf{0} & k_{\bfR}\bfE(\bfR,\bfR^*) \end{bmatrix} \bfM^{-1} \mathbf\frakp_e,
\end{aligned}
\end{equation}
where $\bfE(\bfR,\bfR^*) = \frac{1}{2}\prl{\tr(\bfR^\top \bfR^*) \bfI - \bfR^\top \bfR^* }$ satisfies $\|\bfE(\bfR,\bfR^*)\|_F \leq \sqrt{3}$. Also, by construction of the IDA-PBC controller \cite{duong21hamiltonian}:
\begin{equation}\label{eq:frakpedot}
\dot{\mathbf\frakp}_e = -\bfe - \bfK_d \bfM^{-1} \mathbf\frakp_e - \bfW\bfe_{\bfa}
\end{equation}
Consider the adaptation law $\dot{\bfa} = c_1 \bfW^\top\bfe + c_2 \bfW^\top\bfM^{-1}\mathbf\frakp_e$ in \eqref{eq:geometric_adaptive_law} with $c_1 = c_{\bfp} = c_{\bfR}$ and $c_2 = c_{\bfv}=c_{\bfomega}$ and the Lyapunov function candidate:
\begin{equation} \label{eq:lyapunov_function}
\calV =  \calH_d + \frac{c_1}{c_2} \frac{d}{dt} V_d + \frac{1}{2c_2} \|\bfe_{\bfa}\|_2^2.
\end{equation}
where $V_d$ is the potential energy of the desired Hamiltonian in \eqref{eq:desired_hamiltonian}. The time derivative of $V_d$ satisfies:
\begin{equation}
\frac{d}{dt} V_d = \bfe_{\bfv}^\top \bfe_{\bfp} + \bfe_{\bfomega}^\top \bfe_{\bfR} = \bfe^\top \bfM^{-1} \mathbf\frakp_e.
\end{equation}
For $\bfz := [\|\bfe\|\; \|\mathbf\frakp_e\|]^\top \in \bbR^2$, the Lyapunov function candidate in \eqref{eq:lyapunov_function} is bounded as:
\begin{equation}
\frac{1}{2}\bfz^\top \bfQ_1 \bfz + \frac{1}{2c_2} \|\bfe_{\bfa}\|_2^2 \leq \calV \leq \frac{1}{2}\bfz^\top \bfQ_2 \bfz + \frac{1}{2c_2} \|\bfe_{\bfa}\|_2^2,
\end{equation}
where the matrices $\bfQ_1$ and $\bfQ_2$ are:
\begin{equation}
\begin{aligned}
\bfQ_1 &= \begin{bmatrix} \min\crl{k_{\bfp}, k_{\bfR}} & - \frac{c_1}{c_2} \lambda_{\max}(\bfM^{-1})\\
- \frac{c_1}{c_2} \lambda_{\max}(\bfM^{-1}) & \lambda_{\min}(\bfM^{-1}) \end{bmatrix}\\
\bfQ_2 &= \begin{bmatrix} \max\crl{k_{\bfp}, \frac{2 k_{\bfR}}{2 - \alpha}} & \frac{c_1}{c_2} \lambda_{\max}(\bfM^{-1})\\
\frac{c_1}{c_2} \lambda_{\max}(\bfM^{-1}) & \lambda_{\max}(\bfM^{-1}) \end{bmatrix}.
\end{aligned}
\end{equation}
The time derivative of the Lyapunov candidate satisfies:
\begin{equation*}
\begin{aligned}
\frac{d}{dt}\calV &= \mathbf\frakp_e^\top \bfM^{-1} \dot{\mathbf\frakp}_e +  \bfe^\top \bfM^{-1} \mathbf\frakp_e\\
&\qquad + \frac{c_1}{c_2} \bfe^\top \bfM^{-1} \dot{\mathbf\frakp}_e + \frac{c_1}{c_2} \dot{\bfe}^\top \bfM^{-1} \mathbf\frakp_e + \frac{1}{c_2}\bfe_{\bfa}^\top \dot{\bfa}\\
&= - \mathbf\frakp_e^\top\bfM^{-1}\bfK_{\bfd} \bfM^{-1} \mathbf\frakp_e \\
&\qquad- \frac{c_1}{c_2}\bfe^\top \bfM^{-1}\bfe  -\frac{c_1}{c_2}\bfe^\top \bfM^{-1}\bfK_{\bfd} \bfM^{-1} \mathbf\frakp_e\\
%&\qquad+ \frac{c_1}{c_2} \bfe^\top  \begin{bmatrix} \hat{\bfomega} & \mathbf{0}\\ \mathbf{0}& \mathbf{0} \end{bmatrix} \bfM^{-1} \mathbf\frakp_e\\
&\qquad+ \frac{c_1}{c_2} \bfe^\top  \begin{bmatrix} \hat{\bfe}_{\bfomega} & \mathbf{0}\\ \mathbf{0}& \mathbf{0} \end{bmatrix} \bfM^{-1} \mathbf\frakp_e\\
&\qquad+ \frac{c_1}{c_2} \bfe^\top  \begin{bmatrix} \bfR^\top \bfR^* \hat{\bfomega}^*\bfR^{*\top} \bfR & \mathbf{0}\\ \mathbf{0}& \mathbf{0} \end{bmatrix} \bfM^{-1} \mathbf\frakp_e \\
&\qquad+ \frac{c_1}{c_2} \mathbf\frakp_e^\top \bfM^{-1} \begin{bmatrix} k_{\bfp} \bfI & \mathbf{0}\\\mathbf{0} & k_{\bfR}\bfE(\bfR,\bfR^*) \end{bmatrix} \bfM^{-1} \mathbf\frakp_e,
\end{aligned}
\end{equation*}
where we used \eqref{eq:frakpedot}, \eqref{eq:edot}, and that $\bfomega = \bfe_\bfomega  + \bfR^\top \bfR^* \bfomega^*$ by definition of $\bfe_{\bfomega}$. Hence, on the domain $\calT$, we have:
\begin{equation}
\frac{d}{dt}\calV \leq - \bfz^\top \bfQ_3 \bfz = - \bfz^\top \begin{bmatrix} q_1 & q_2 \\ q_2 & q_3\end{bmatrix}\bfz,
\end{equation}
where the elements of $\bfQ_3$ are:
\begin{equation*}
\begin{aligned}
q_1 &= \frac{c_1}{c_2} \lambda_{\min}(\bfM^{-1}),\\
q_2 &= -\frac{c_1}{c_2} \prl{ \lambda_{\max}(\bfM^{-1}\bfK_{\bfd}\bfM^{-1}) + \beta + \gamma \lambda_{\max}(\bfM^{-1})},\\ 
q_3 &= \lambda_{\min}(\bfM^{-1}\bfK_{\bfd}\bfM^{-1}) - \frac{c_1}{c_2} \max\crl{k_{\bfp},\sqrt{3}k_{\bfR}}\lambda_{\max}^2(\bfM^{-1}).
\end{aligned}
\end{equation*}
Since $k_{\bfp}$, $k_{\bfR}$, $\bfK_{\bfd} = \diag(k_{\bfv}\bfI,k_{\bfomega}\bfI)$ can be chosen arbitrarily large, there exists some choice of parameters that ensures that the matrices $\bfQ_1$, $\bfQ_2$, and $\bfQ_3$ are positive definite. By the LaSalle-Yoshizawa theorem \cite[Thm.~A.8]{krstic1995nonlinear}, the tracking errors $\bfe$, $\mathbf\frakp_e$ are asymptotically stable, while the estimation error $\bfe_{\bfa}$ is stable and uniformly bounded. 
\end{proof}
